# Supplementary material for: Dynamics of cascades on burstiness-controlled temporal networks
Source: arXiv:2007.06223 source file (2020-07-13)
Supplement: Supplementary file 2 [file supplementary_preamble.tex]

% table of contents, disable subsections
\makeatletter
\def\l@subsection#1#2{}
\def\l@subsubsection#1#2{}
\makeatother

% table of contents, change name
\renewcommand{\tocname}{C\lowercase{ontents}}

\newcommand{\seref}[1]{Supplementary Eq.~(\ref{#1})}
\newcommand{\serefs}[2]{Supplementary Eqs.~(\ref{#1}) and (\ref{#2})}
\newcommand{\sfref}[1]{Supplementary Fig.~\ref{#1}}
\newcommand{\sfrefs}[2]{Supplementary Figs.~(\ref{#1}) and (\ref{#2})}
\newcommand{\stref}[1]{Supplementary Table~\ref{#1}}

% prefix for figure names
\renewcommand\figurename{\text{Supplementary Figure}}
\renewcommand\thefigure{\text{\arabic{figure}}}

% prefix for table names
\renewcommand\tablename{\text{Supplementary Table}}

% override default revtex enumeration of sections
\newcounter{suppnote}
\refstepcounter{suppnote}

% Supplementary Notes
\newcommand{\SN}{\lowercase{\uppercase{S}upplementary \uppercase{N}ote}}
\newcommand{\SNmaster}{Supplementary Note 1} % 1. Master equation solution    
\newcommand{\SNstationary}{Supplementary Note 2} % 2. Random walk equivalence
\newcommand{\SNsimulating}{Supplementary Note 3} % 3. Monte Carlo simulation
\newcommand{\SNlaplace}{Supplementary Note 4} % 4. Laplace transform inversion
\newcommand{\SNexternal}{Supplementary Note 5} % 5. Diffusion speed and noise
\newcommand{\SNexplicit}{Supplementary Note 6} % 6. Comparing diffusion times
\newcommand{\SNeffectiveness}{Supplementary Note 7} % 7. Mean field approximation
\newcommand{\SNprobability}{Supplementary Note 8} % 8. Probability distributions

% figures in the main text
\newcommand{\MTmirror}{Fig. 1}
\newcommand{\MTheat}{Fig. 2}
\newcommand{\MTcollapse}{Fig. 3}
